# Supplementary material for: Steering LLMs toward Korean Local Speech: Iterative Refinement Framework for Faithful Dialect Translation
Source: arXiv:2511.06680 source file (2026-03-17)
Supplement: Supplementary file 2 [file prompt2.tex]

% fig_prompt_zero_shot.tex
\begin{figure*}[t]
\centering
\begin{promptbox}
Input sentence: {SOURCE}
Translation:
\end{promptbox}
\caption{Zero-shot prompt templet.}
\label{fig:prompt-2-zero-shot}
\end{figure*}
