# Supplementary material for: Steering LLMs toward Korean Local Speech: Iterative Refinement Framework for Faithful Dialect Translation
Source: arXiv:2511.06680 source file (2026-03-17)
Supplement: Supplementary file 3 [file prompt3.tex]

% fig_prompt_icl.tex  (listings 기반 promptbox에서 안전)
\begin{figure*}[t]
\centering
\begin{promptbox}
Example:
A: {STANDARD_EXAMPLE_1}
B: {DIALECT_EXAMPLE_1}

Example:
A: {STANDARD_EXAMPLE_2}
B: {DIALECT_EXAMPLE_2}

... (total of 10 examples)

Input sentence: {SOURCE}
Translation:
\end{promptbox}
\caption{In-context learning prompt templet.}
\label{fig:prompt-3-icl}
\end{figure*}
