# Supplementary material for: Steering LLMs toward Korean Local Speech: Iterative Refinement Framework for Faithful Dialect Translation
Source: arXiv:2511.06680 source file (2026-03-17)
Supplement: Supplementary file 5 [file prompt5.tex]

% fig_prompt_cil_oscillation.tex
\begin{figure*}[t]
\centering
\begin{promptbox}
The output oscillates between {last_wrong_label} and {wrong_label}. Please make the {dialect}-specific features more explicit.
\end{promptbox}
\caption{Oscillation prompt template. Used in \texttt{DIA-REFINE}; when the two most recent hypotheses are misclassified into different non-target dialects, it is inserted into the feedback prompt to flag oscillation and help the model break the cycle and steer generation toward the target dialect.}
\label{fig:prompt-cil-oscillation}
\end{figure*}
